# Supplementary material for: Understanding Queries by Conditional Instances
Source: arXiv:2202.11160 source file (2022-02-22)
Supplement: Supplementary file 1 [file appendix--old.tex]

\appendix
\section{Appendix}\label{sec:appendix}


\subsection{Proof of completeness in Section \ref{sec:analysis}}

The proof of Theorem~\ref{theorem:completeness} needs Lemma~\ref{lemma:union-c-homo}, Lemma~\ref{lemma:and-sat}, and Lemma~\ref{lemma:forall-sat}.

\begin{Lemma}\label{lemma:union-c-homo}
Given two c-instances $J_1$ and $J_2$ that c-homomorphically map to a ground instance $K$ under $\assignment_1$ and $\assignment_2$ respectively, if for every $x \in vars(J_1) \cap vars(J_2)$, $\assignment_1(x) = \assignment_2(x)$, $J_1 \cup J_2$ c-homomorphically maps to $K$ under $\assignment_1 \cup \assignment_2$.
\end{Lemma}

\begin{proof}
We show that $\assignment = \assignment_1 \cup \assignment_2$ is a c-homomorphism from $J_1 \cup J_2$ to $K$. Let $\phi \in J_1 \cup J_2$ be an arbitrary relational atom $\rel(x_1, ..., x_{\relarity})$, by the definition of c-homomorphism, $K$ contains $\rel(\assignment(x_1), ..., \assignment(x_{\relarity}))$; let $\phi$ be the negation of an arbitrary relational atom $\neg \rel(x_1, ..., x_{\relarity})$, $K$ does not contain the relational fact  $\rel(\assignment(x_1), ..., \assignment(x_{\relarity}))$, and thus $\assignment(J_1 \cup J_2)$ does not contain $\rel(\assignment(x_1), ..., \assignment(x_{\relarity}))$; let $\phi \in J_1 \cup J_2$ be an arbitrary binary expression $x~op~y$, we also have the image under $\assignment$ of this expression $\assignment(x)~op~\assignment(y)$ to be True in $K$. Hence $J_1 \cup J_2$ c-homomorphically maps to $K$ under $\assignment_1 \cup \assignment_2$. \SR{polish}
\end{proof}

\begin{Lemma}\label{lemma:and-sat}
Given a DRC query $Q=Q_1 \land Q_2$, a ground instance $K$ that satisfies $Q$, and two c-instances $J_1$ and $J_2$ that c-homomorphically map to $K$ and satisfy $Q_1$ and $Q_2$ respectively, if either $Q_1$ or $Q_2$ has no quantifiers, then $J_1 \cup J_2$ c-homomorphically map to $K$ and satisfies $Q$.
\end{Lemma}

% \begin{Lemma}\label{lemma:union-coverage}
% Given two c-instances $J_1$ and $J_2$ that c-homomorphically map to a ground instance $K$ under $h_1$ and $h_2$ respectively and a syntax query tree $Q$ where $J_1$ and $J_2$ satisfy $Q$ with coverage $\cov_1$ and $\cov_2$ respectively, $J_1 \cup J_2$ satisfies $Q$ 
% \end{Lemma}

\begin{Lemma}\label{lemma:forall-sat}
Given a DRC query $Q=\forall x Q'(x)$, a ground instance $K$ that satisfies $Q$, and $l$ c-instances $J_1, J_2, ..., J_l$ that c-homomorphically map to $K$ and satisfy $h_i(Q')$ respectively, where $l = |K.dom(x)|$ and each $h_i$ maps the free variable $x$ in $Q'$ to a different value in $K.dom(x)$, if either $Q_1$ or $Q_2$ has no quantifiers, then there exist c-instances $J'_1, J'_2, ..., J'_l$ such that each $J_i$ homomorphically maps to $J'_i$ and $\bigcup_{i=1}^{l} J'_i$) c-homomorphically maps to $K$ and it satisfies $Q$.
\end{Lemma}

\begin{proof}[Proof for Theorem~\ref{theorem:completeness}]
We prove the theorem by induction of the number of nodes in the syntax tree $Q$. 

%\zhengjie{safety issue here}
If $|V(Q)| = 1$, there is only one leaf node $u$ --- it can only be an atom or the negation of an atom \SR{do you keep the $\neg$? see defn 11}, and the coverage can only be $\{u.atom\}$ (otherwise $Q$ evaluates to an empty result), and the homomorphism $h$ maps the free variables in $u.atom$ to vales in $K$, i.e., $h(u.atom)$ exists in $J$ if it is a relational atom, or it evaluates to True otherwise.
In this case, the algorithm simply calls $\proc{RD-Tree-Chase}$ one time to add this atom to the empty c-instance and returns a list with only this instance, which covers $u.atom$. $h$ is the c-homomorphism from the variables in $u.atom$ to values in $K$.

\amir{Change the induction hypothesis to make the coverages equal and not contained:} Assume that for every $Q$ such that $|V(Q)| < n$, for a ground instance $K$ satisfying $Q$ with coverage $\cov$ under a homomorphism $h$, there is a c-instance in the result of Algorithm~\ref{alg:rd-tree-chase-main} has coverage $\cov' \supseteq \cov$ for $Q$ that c-homomorphically maps to $K$. We show that the claim is true for $Q$ with $|V(Q)| = n$.

If the root of $Q$ is an $\land$ node, i.e., $Q = Q_1 \land Q_2$ where $V|Q_1| < n$ and $V|Q_2| < n$, and then the coverage of $K$ for $Q$ is $\cov = \cov_1 \cup \cov_2$ where $\cov_1$ is a subset of leaf atoms of $Q_1$ and $\cov_2$ is a subset of leaf atoms of $Q_2$.  Since the tree $Q$ is a right deep syntax tree, its left child $Q_1$ has no quantifiers (has only connecitves and leaf atoms), in lines 14 it directly generates a list of conjunction of atoms from $Q_1$ by expanding disjunctions into three conjuncive cases ($A \lor B \to \{A \land B, A \land \neg B, \neg A \land B$\}), then any $\cov_1$ of $Q_1$ must be covered in one of the expanded conjunctions. Furthermore, note that keep running the procedure $\proc{RD-Tree-Chase}$ in Algorithm~\ref{alg:rd-tree-chase-main} does not change the results on $Q_1$ --- the free variables are all assigned fresh variables at the beginning of Algorithm~\ref{alg:rd-tree-chase-main}, and thus it does not add new variables to the domain of the c-instances. 
Therefore, we run Algorithm~\ref{alg:rd-tree-chase-main} on $Q$ as running Algorithm~\ref{alg:rd-tree-chase-main} on $Q_1$ and $Q_2$ separately, and then merging the result instances from $Q_1$ to the result instances from $Q_2$. %In line 15-16, we write it as a recursive call to $\proc{RD-Tree-Chase}$ on the right child $Q_2$ of $Q$ for each of the expanded conjunction from $Q_1$. 
% \amir{I wasn't able to follow this argument. Can't there be an intersection between the domains considered in $Q_1$ and those considered in $Q_2$? e.g., if the root of $Q_2$ is a universal quantifier that applies to the vars in $Q_1$}. 
%Since there must be a expanded conjunction from $Q_1$ with coverage $\cov_1$, and by

\begin{figure}[h]
\centering
 \includegraphics[width=.8\linewidth]{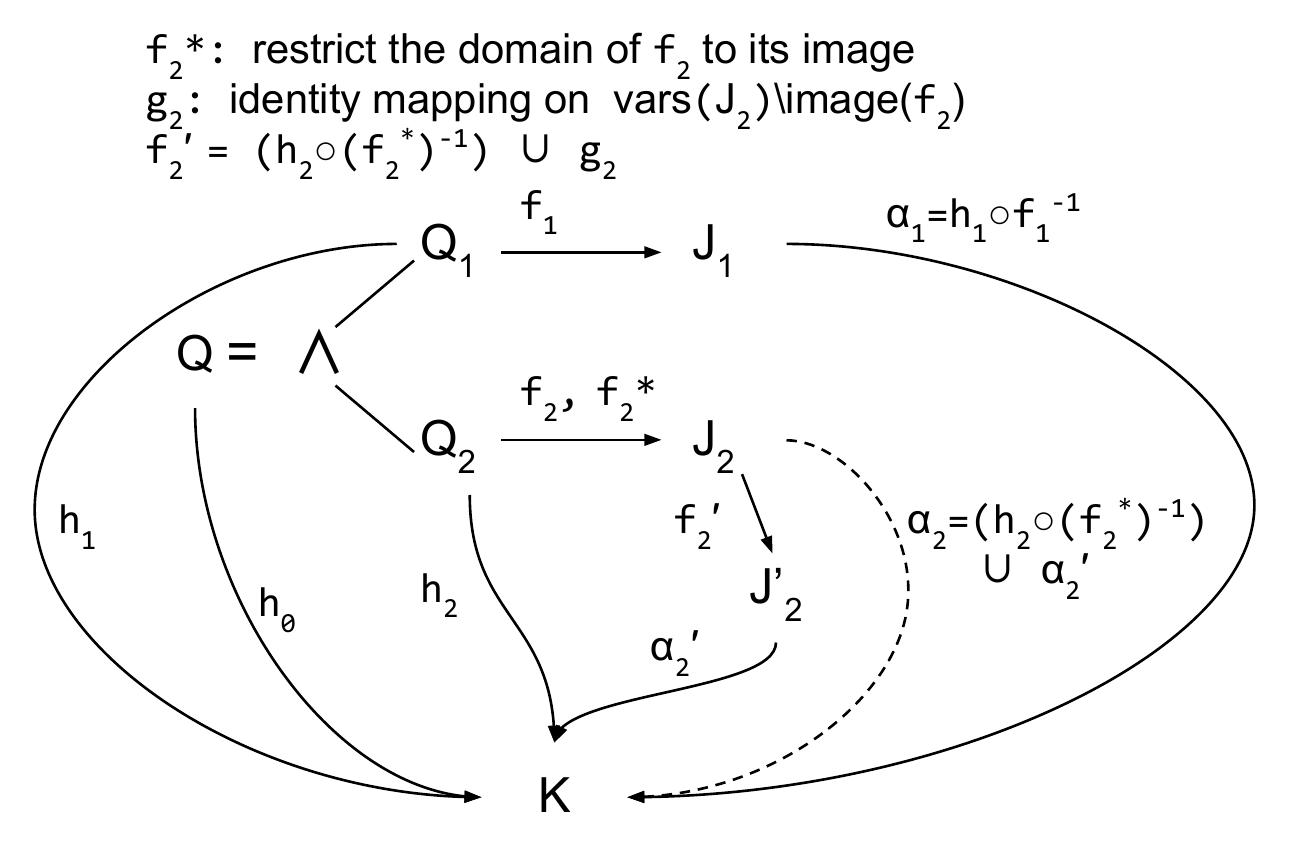}
  \caption{Illustration of the $\land$ case in Proof of Theorem~\ref{theorem:completeness}}
  \label{fig:proof-completeness-and}
\end{figure}
By the induction hypothesis, since $K$ satisfies $Q_1$ and $Q_2$ with coverage $\cov_1$ and $\cov_2$ respectively, there are a c-instance $J_1$ for $Q_1$ with coverage $\cov_1' \supseteq \cov_1$ and a c-instance $J_2$ for $Q_2$ with coverage $\cov_2' \supseteq \cov_2$ in the results of Algorithm~\ref{alg:rd-tree-chase-main}, and both $J_1$ and $J_2$ c-homomorphically map to $K$ under $\assignment_1$ and $\assignment_2$ respectively.
% \amir{But $K$ can be satisfiable without $J_1$/$J_2$ being satisfiable, right? ($K$ is always satisfied because its grounded)}. 
We next show that there is are two mappings between $J_1$ and $J_2$ to $K$ respectively, such that their union maps $J_1 \cup J_2$ to $K$. 

Because $K$ satisfies $Q=Q_1 \land Q_2$, there exists a homomorphism $h_0$ that maps free variables in $Q_1 \land Q_2$ to values in $K$, such that $K$ satisifies $Q_1 \land Q_2$ under $h_0$. In particular, $K$ satisfies $Q_1$ and $Q_2$ so the induction hypothesis can be used. 
Hence, we have $h_1 = h_0|_{vars(Q_1)}$ that maps the free variables in $Q_1$ to values in $K$, and $h_2 = h_0|_{vars(Q_2)}$ maps the free variables in $Q_2$ to values in $K$.
We show that we can construct c-homomorphsims $\assignment_1$ and $\assignment_2$ that have no conflicts. Suppose $f_1$ and $f_2$ are the mappings from free variables in $Q_1$ and $Q_2$ to variables in $J_1$ and $J_2$ respectively, as initialized in Algorithm~\ref{alg:rd-tree-chase-main} to be identity functions. Hence for $Q_1$ we have $\assignment_1 = h_1 \circ f_1^{-1}$ to be a c-homomorphism from $J_1$ to $K$ (since the algorithm assigns fresh variables to all free variables in $J_1$ in lines \ref{l:iter-free}--\ref{l:add-fresh}, $f_1$ is bijective and therefore $f_1^{-1}$ is a mapping from $J_1$ to free variables in $Q_1$). For $Q_2$, we build two mappings 
%$h_2^{**}: x \to h_2^*(x)$ 
%$h_2^{**-1}: h_2^*(x) \to x$
$(f_2^{*})^{-1}: Im(f_2) \to FreeVars(Q_2)$
by restricting the co-domain of $f_2$ to its image and an identity function $g_2: vars(J_2)\setminus image(f_2) \to vars(J_2)\setminus image(f_2)$, then we construct $f'_2 = (h_2 \circ f_2^{*-1}) \cup g_2$ maps variables in the image of $f_2$ to values in $K$ and keeps other variables in $J_2$ unchanged. Then the c-instance $J_2' = f'_2(J_2)$ satisfies $f_2(Q_2)$ with coverage contains $f_2(C_2)$ (we abuse $f_2$ here, i.e., only free variables in $Q_2$ are mapped to values in $K$ while other variables and constants are not changed) \amir{Did not follow this. $h_2^*(Q_2)$ is a c-instance, not a query, right?}. Again by the induction hypothesis, $J_2'$ c-homomorphically maps to $K$ under some $\assignment_2'$, then we have $\assignment_2 =  (h_2 \circ f_2^{*-1}) \cup \assignment_2'$ is a c-homomorphsim from $J_2$ to $K$. 

Now we show that $J_1 \cup J_2$ c-homomorphically maps to $K$ and covers $Q_1 \land Q_2$ with coverage $\cov' \supseteq \cov_1 \cup \cov_2$. 
The former is directly by Lemma~\ref{lemma:union-c-homo}: since $h_1'$ and $h_2'$ \amir{$h_1$ and $h_2$?} agree on all variables in the intersection of their domains (variables that can be mapped from the free variables), implying that $h_1$ and $h_2$ have no conflicts, therefore $J_1 \cup J_2$ c-homomorphically maps to $K$. 
% The former is directly by the fact that $h_0$ is a c-homomorphism from $J_1$ to $K$ and $h_2 \circ h_0$ is a c-homomorphism from $J_2$ to $K$.
% Let $\phi \in J_1 \cup J_2$ be an arbitrary relational atom, by the definition of c-homomorphism, $K$ contains $(h_2 \circ h_0)(\phi)$; let $\phi$ be the negation of an arbitrary relational atom, $K$ does not contain the relational fact of $(h_2 \circ h_0)(\phi)$; let $\phi \in J_1 \cup J_2$ be an arbitrary binary expression $x op y$, we also have the image under $h_2 \circ h_0$ of this expression $(h_2 \circ h_0)(x) op (h_2 \circ h_0)(y)$ to be True in $K$. Hence $J_1 \cup J_2$ c-homomorphically maps to $K$ under $h_2 \circ h_0$. 

For the claim on coverage, assume $J_1 \cup J_2$ does not satisfy $Q$ with coverage $\cov' \supseteq \cov$. Since $Q_1$ has no quantifiers, $J_1 \cup J_2$ must satisfy $Q_1$ with coverage $\cov'_1 \supseteq \cov_1$ (the c-homomorphism $\assignment_1 \cup \assignment_2$ also gives an assignment for $J_1 \cup J_2$ that satisfies $Q_1$); and since $J_1 \cup J_2$ c-homomorphically maps to $K$, $J_1 \cup J_2$ is consistent, then the only case is that there is an atom $\beta \in \cov_2$ is covered by $J_2$ but not by $J_1 \cup J_2$. That is, the insertion of some atoms in $J_1$ into $J_2$ makes $\beta$ not homomorphically map to some atom in $J_2$, which is impossible \amir{Couldn't $\beta$ be a condition that has a conflict with $J_2$?}. Hence, the assumption is wrong, $J_1 \cup J_2$ satisfies $Q$ with coverage $\cov' \supseteq \cov$.
 
If the root of $Q$ is an $\lor$ node, i.e., $Q = Q_1 \lor Q_2$ where $V|Q_1| < n$ and $V|Q_2| < n$, and then the coverage $\cov = \cov_1 \cup \cov_2$ where $\cov_1$ is a subset of leaf atoms of $Q_1$ and $\cov_2$ is a subset of leaf atoms of $Q_2$. The algorithm splits the tree into three cases, where each is rooted by a $\land$ node: (1) where no child of the root is negated, (2) where the left child is negated and (3) where the right child is negated. Then it is reduced to the above $\land$ case.

If the root of $Q$ is an $\exists$ node: $Q = \exists x Q'(x)$ where $V|Q'| < n$, 
it is clear that if $\cov$ is covered by some instance $K$ for $Q$, then it is also covered by $K$ for $Q'$. By the induction hypothesis, there is a c-instance $J$ outputted by Algorithm~\ref{alg:rd-tree-chase-main} for $Q'$ with coverage containing $\cov$ that c-homomorphically maps to $K$, and $J$ is also a satisfying c-instance for $Q$ with coverage containing $\cov$.

If the root of $Q$ is an $\forall$ node: $Q = \forall x Q'(x)$ where $V|Q'| < n$, $\cov$ is covered by $K$ for $Q$ under homomorphism $h$. Unlike the above $\exists$ case, for $Q'$, different subsets of $\cov$ (denoted as $\cov_1, ..., \cov_l$, where \cov = $\bigcup_{i=1}^{l}\cov_i$) are covered under different homomorphisms that map the free variable $x$ to different values $v_i$ in the domain of $x$ in $K$. 

We show by construction that a c-instance that c-homomorphically maps to $K$ and satisfies $Q$ with coverage $\cov' \supseteq \cov$ will be outputted by Algorithm~\ref{alg:rd-tree-chase-main}.
For each value in $K$ we create a corresponding variable to obtain a c-instance $J_0$ with an empty global condition \amir{lines?}, and denote the bijection from the variables in $J_0$ to the values in $K$ as $\assignment$ (we also abuse $\assignment$ as a homomorphism from $J_0$ to $K$, $\assignment(J_0) = K$, $\assignment^{-1}(K) = J_0$).
Then, we initialize the c-instance $I_0$ in Algorithm~\ref{alg:rd-tree-chase-main} by setting its domains to be the same as $J_0$ \amir{lines?}. That is, when running the algorithm, instead of allowing the algorithm to create fresh variables, we skip lines \ref{alg:rd-tree-chase:line:exists-add-fresh-start}-\ref{alg:rd-tree-chase:line:exists-add-fresh-end}, \ref{alg:rd-tree-chase:line:forall-add-fresh-start}-\ref{alg:rd-tree-chase:line:forall-add-fresh-end} in Algorithm~\ref{alg:rd-tree-chase} and thus only allow it to map the quantified variables to one of the variables added in advance in $J_0$.

For each coverage subset $\cov_i$, we define a mapping $h_i = h \cup \{x \to v_i\}$ where $x$ is the quantified variable at the root of $Q$ and value $v_i \in K.\dom(x)$, then $h_i$ maps the free variables in $Q'$ to values in $K$, i.e., $K$ satisfies $Q'$ with coverage $\cov_i$ under $h_i$.

\begin{figure}[h]
\centering
 \includegraphics[width=.6\linewidth]{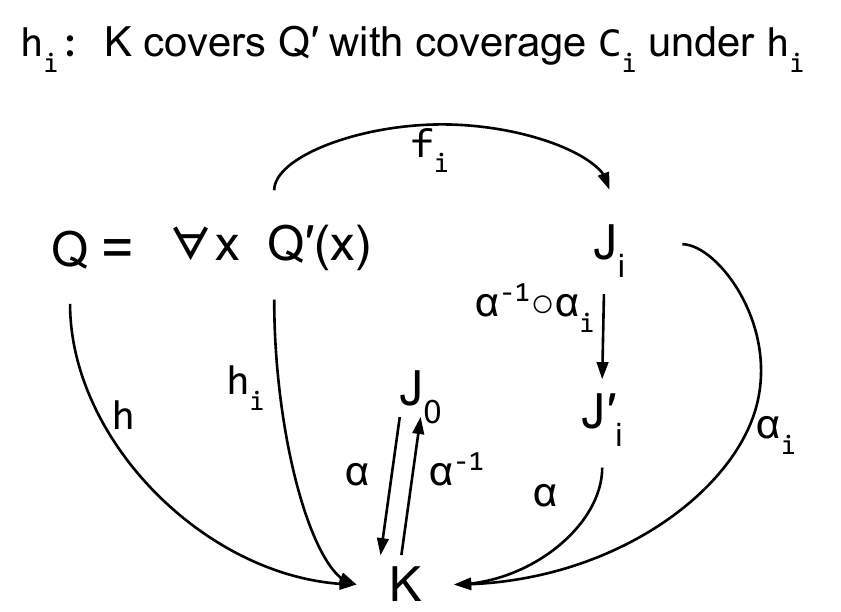}
  \caption{Illustration of the $\forall$ case in Proof of Theorem~\ref{theorem:completeness}}
  \label{fig:proof-completeness-forall}
\end{figure}

By the induction hypothesis, for each $v_i$, since the ground instance $K$ covers $Q'$ with coverage $\cov_i$ under $h_i$, there is a c-instance $J_i$ outputted by Algorithm~\ref{alg:rd-tree-chase-main} that satisfies both $Q'$ with coverage $\cov'_i \supseteq \cov_i$ and c-homomorphically maps to $K$ under some $\assignment_i$. Since $\assignment$ is a bijection, let $J'_i = \assignment^{-1}(\assignment_i(J_i))$, then $J'_i$ also covers $Q'$ with coverage $\cov'_i$ \amir{explain why $J'_i$ is different from $J_0$}. Because each $J'_i$ is mapped to a sub-instance of $K$ under $\assignment$, the union of all $J'_i$-s ($J = \bigcup_{i=1}^{l} J'_i$) c-homomorphically maps to $K$ under $\assignment$ and thus it satisfies $Q$ with coverage $\cov' \supseteq \cov$. 

The original algorithm can find such $J = \bigcup_{i=1}^{l} J'_i$, because (1) the algorithm dynamically increases the size of each domain and will reach the same cardinality in all domains as $J_0$, and (2) each ideal $J'_i$ will be returned the algorithm (line 51-53 in Algorithm~\ref{alg:rd-tree-chase}) --- from the construction procedure above we know that the difference between each $J_i$ and $J'_i$ is that they may contain a different subset of variables in $J_0$, however, since the Algorithm~\ref{alg:rd-tree-chase} will enumerate every variable in the domain when dealing with quantified variables, every possible subset of variables in $J_0$ will be considered. Therefore, whenever there is a valid $J = \bigcup_{i=1}^{l} J'_i$, the algorithm will find it.

% Now we show the union of all $J'_i$-s ($J = \bigcup_{i=1}^{l} J_i$) c-homomorphically maps to $K$ and satisfies $Q$ with coverage $\cov' \supseteq \cov$. First, for each $J_i$ and $h_i$, we create a new variable $x_i$ to replace the universally quantified $x$ in $Q$ (remember that free variables are directly added to the domain of the c-instances). 
% Then, in each $J_i$, we rename all variables such that there are no shared variables in all $J_i$-s except the free variables in $Q$.
% To do this, in $\proc{RD-Tree-Chase}$, we set the domain of $x$ to be $\{x_1, ..., x_l\}$ (changee line 44) and do not create fresh variables for $x$ (line 34-37 and line 54-60 are skipped for the domain of $x$), and rename the variables in the resulting c-instances of the recursive call of $\proc{RD-Tree-Chase}$ for each variable in the domain (line 48-53), such that there are no shared variables except the free variables in $Q$. Because all $h_i$-s are extensions of $h$, by Lemma~\ref{lemma:union-c-homo}, $J$ c-homomorphically maps to $K$ under $h' = \bigcup_{i=1}^{l} h_i$.

% For the claim on coverage, assume that for some $Q'_i$, there is an atom $\beta \in \cov_i$ not covered by $J$ but covered by $J_i$. By definition, there exists some homomorphism that maps $\beta$ to an atom in $J_i$, and such an atom still appear in $J$. 

For cases where the syntax tree is negated, the algorithm will change the root operator accordingly ($\land$ to $\lor$, $\land$ to $\lor$, $\exists$ to $\forall$, and $\forall$ to $exists$) and change the negated flags of the root and the children. 
\end{proof}


% \subsection{Proofs of soundness in Sections \ref{sec:analysis}}



\subsection{Auxiliary Methods}
\amir{Add description for each method}


\begin{algorithm}[h]\caption{Auxiliary Methods}\label{alg:auxiliary}
  \centering
{\small

% \MyStruct{Node}{
%   Node* parent\;
%   int size\;
%   \tcp{other stuff}
% }
\begin{algorithmic}[1]
\Procname{The Structure of C-Instance}\label{alg:structure-cins}
\State Structure of \proc{C-Instance} $\{$
\State \quad domain: sets of variables for each domain;
\State \quad $\rel_1, \rel_2, ..., \rel_{\relnum}$: c-tables of each relation;
\State \quad conditions: list of atoms
\State  $\};$
\end{algorithmic}
\begin{codebox}
\algorithmicrequire $\schemaOf{\rel}$: the schema of the relational database;\\
$I$: a c-instance; $\phi$: a conjunction of literals.\\
\algorithmicensure a c-instance\\
  \Procname{$\proc{Add-to-Ins}(\schemaOf{\rel}, I, \phi)$}
  \li $J \gets \text{CopyOf}(I)$
  \li \For each literal $\omega \in \phi$
  \Do
  \li \If $\omega = \rel_i(y_1, ..., y_\relarity)$
    \Then
        \li \If $(y_1, ..., y_\relarity) \notin J.\rel_i$ 
        \Then \li Add a new row$(y_1, ..., y_\relarity)$ to $J.\rel_i$  
        \End
    \li \Else
        \li \If $\omega \notin J.conditions$ 
        \Then \li Add $\omega$ to $J.conditions$ 
        \End
    \End
  \End
  \li \Return $J$
  \label{alg:add-to-ins}
 \end{codebox}
 
%  \begin{codebox}
% \label{alg:add-fresh-var}
% \algorithmicrequire 
% $I$: a c-instance; $x$: a quantified variable in the syntax tree.\\
% \algorithmicensure a fresh variable\\
%   \Procname{$\proc{Add-Fresh-Var}(I, x)$}
%   \li Create a fresh variable $y$ in the domain of $x$
%   \li $I.domain(x) \gets I.domain(x) \cup \{y\}$
%   \li \Return $y$
%  \end{codebox}

\begin{codebox}
\algorithmicrequire $T$: a syntax tree of a DRC query with no disjunctions.\\
\algorithmicensure a c-instance\\
  \Procname{$\proc{conjtree-to-conj}(Q)$}
  \li $res \gets []$
  \li \If T is null
  \Then
    \li \Return $res$
  \End
  \li \If T.root is an atom
  \Then
    \li $res.append(T.root.atom)$
  \li \ElseIf T.root.operator $\in \{\land\}$
    \li $res \gets \proc{conjtree-to-conj}(T.root.left)$
    \li $res.extend(\proc{conjtree-to-conj}(T.root.right))$
  \End
  \li \Return $res$
\label{alg:conjtree-to-conj}
 \end{codebox}
 
\begin{codebox}
\algorithmicrequire 
$Q$: a syntax tree of a DRC query.\\
\algorithmicensure a list of conjunctive predicates\\
  \Procname{$\proc{tree-to-conj}(Q)$}
  \li $ConjTrees \gets \proc{disjtree-to-conjtrees}(Q)$
  \li $res \gets []$
  \li \For each $t \in ConjTrees$
  \Do
    \li $res.append(\proc{conjtree-to-pred}(t))$
  \End
  \li \Return $res$
  \label{alg:tree-to-conj}
 \end{codebox}

\begin{codebox}
\algorithmicrequire 
$Q$: a syntax tree of a DRC query rooted at $\lor$.\\
\algorithmicensure a list of syntax query trees rooted at $\land$\\
  \Procname{$\proc{Expand-DisjTree}(Q)$}
   \li T $\gets$ CopyOf(Q)
   \li T.root.lchild.negated $\gets$ Q.root.lchild.negated
    \li T.root.rchild.negated $\gets$ Q.root.rchild.negated
    \li res $\gets$ [T]
    \li T.root.lchild.negated $\gets$ Q.root.lchild.negated
    \li T.root.rchild.negated $\gets \neg$ Q.root.rchild.negated
    \li res.append(T)
    \li T.root.lchild.negated $\gets \neg$ Q.root.lchild.negated
    \li T.root.rchild.negated $\gets$ Q.root.rchild.negated
    \li res.append(T)
    \li res.expand([Q.root.lchild,  Q.root.rchild])
  \li \Return $res$
  \label{alg:tree-to-conj}
 \end{codebox}
}
\end{algorithm}


\subsection{Checking Satisfaction of Syntax Trees}\label{sec:tree-sat}
\amir{Add description for the algo.}

\begin{algorithm}[t]\caption{Tree-Satisfied}\label{alg:tree-sat}
{\small
\begin{codebox}
\algorithmicrequire
$Q$: a syntax tree of a DRC query; \\
$I$: current c-instance; \\
$f$: current mapping from $var(Q)$ to $var(I) \cup cons(I)$.\\
\algorithmicensure True if $I$ satisfies $Q$; False otherwise \\
  \Procname{$\proc{Tree-SAT}(Q, I, f)$}
  \li \If $Q$ has free variables
  \Then
    \li \For $x \in FreeVar(Q)$
      \Do
          \li $Q \gets \exists x Q(x)$
      \End
  \End
  \li \If Q.root is an atom
  \Then 
    \li \If Q.negated
    \Then 
        \li Q.root.atom $\gets \neg$ Q.root.atom
    \End
    \li \If $f(Q.root.atom) \in I$ 
        \Then
            \li \Return True\label{l:root_in_instance}
        \li \Else
            \li \Return False
        \End
  \End
  \li \If Q.root.operator $\in \{\land\}$
  \Then
    \li \Return $\proc{Tree-SAT}(Q.root.lchild, I, f) \land $ $\proc{Tree-SAT}( Q.root.rchild, I, f)$\label{l:recurse_and}
 \li \ElseIf Q.root.operator $\in \{\lor\}$
  \Then
    \li \Return $\proc{Tree-SAT}(Q.root.lchild, I, f) \lor $ $\proc{Tree-SAT}( Q.root.rchild, I, f)$\label{l:recurse_or}
  \li \ElseIf Q.root.operator $\in \{\exists\}$
  \Then
    \li \For $x \in I.domain(Q.root.variable)$
    \Do
        \li $g \gets f \cup \{Q.root.variable \to x\}$
        \li \If $\proc{Tree-SAT}( Q.root.child, I, g)$ 
        \Then
            \li \Return True\label{l:exists_in_instance}
        \End
    \End
    \li \Return False
  \li \ElseIf Q.root.operator $\in \{\forall\}$
  \Then 
    \li \For $x \in I.domain(Q.root.variable)$
    \Do
        \li $g \gets f \cup \{Q.root.variable \to x\}$
        \li \If $not\ \proc{Tree-SAT}( Q.root.child, I, g)$ 
        \Then
            \li \Return False
        \End
    \End
    \li \Return True\label{l:all_mappings_in_instance}
  \End
\end{codebox}
}
\end{algorithm}


\begin{proposition}\label{prop:soundness-conj-sat}
Given $R$, $I$, and $Q$, Algorithm~\ref{alg:tree-sat} returns True for $Q$ and $I$ iff $I$ satisfies $Q$.
\end{proposition}

\begin{proof}
($\rightarrow$) Assume Algorithm~\ref{alg:tree-sat} returns True for some $Q$ and $I$. 
We prove that $Q$ is satisfied by $I$ using induction over the size of $Q$. 
If $Q$ is of size $1$, then the algorithm returns True in line \ref{l:root_in_instance} after checking that the only node in $Q$ is included in $I$. 
For the induction hypothesis, assume that for every $Q$ of size $< n$, Algorithm~\ref{alg:tree-sat} returns True for $Q$ and $I$ if $I$ satisfies $Q$. Now, suppose $Q$ is of size $n$. 
If Algorithm~\ref{alg:tree-sat} returns True in line \ref{l:recurse_and}, this means that the root of $Q$ is an $\land$ node and, according to the induction hypothesis, both the left and right subtrees of $Q$ are satisfied by $I$. Thus, $Q$ is also satisfied by $Q$. 
If Algorithm~\ref{alg:tree-sat} returns True in line \ref{l:exists_in_instance}, the root of $Q$ is an $\exists$ quantifier. Then, in line \ref{l:iter_demain_exists} the algorithm iterates over the domain of the quantified variable, adds it to the mapping list and checks whether replacing the quantified variable with its current mapping satisfies both the right and left subtrees rooted at the children of the $\exists$ quantifier (this check is correct according to the induction hypothesis). In this case, one of the mappings satisfies both subtrees, and therefore satisfies $Q$.
If Algorithm~\ref{alg:tree-sat} returns True in line \ref{l:all_mappings_in_instance}, according to the induction hypothesis, for all mappings of the variable $x$ to constants/variables in its domain, the tree in which $x$ is mapped to a constant/variable satisfies $Q$ and therefore, the tree with the $\forall~x$ node satisfied $Q$. 

($\leftarrow$) Now, suppose $I$ satisfies $Q$. We show that Algorithm~\ref{alg:tree-sat} will return True. 
This again will be proven by induction on the size of $Q$. 
If $Q$ is of size $1$, the algorithm checks whether the single node in $Q$ is in $I$ and returns True iff it is. 
Assume that if $Q$ is of size $< n$ and $I$ satisfies $Q$, then Algorithm~\ref{alg:tree-sat} will return True. We prove the claim for $Q$ of size $n$. 
\amir{this is very similar to the first direction.}
\end{proof}


\subsection{Complexity Results}\label{sec:complexity}
\amir{Verify}

\begin{table}[t]
\begin{small}
\centering
\caption{Complexity of finding a universal solution}\label{tab:complexity}
\begin{tabularx}{\linewidth}{| c | >{\centering\arraybackslash}X | c |}
\hline Query Class & Operators & Complexity/Compatibility\\
\hline $CQ_{\neg}$ & $\land$,$\exists$, $\neg$ for individual atoms and cond. & $P$\\
\hline $UCQ_{\neg}$ & $\land$, $\exists$, $\lor$, $\neg$ for individual atoms and cond. & $\#P$-complete\\
\hline $DRC$ & $\land$, $\exists$, $\neg$, $\lor$, $\forall$ & $\mathcal{RE} \setminus \mathcal{R}$ (undecidable)\\
\hline
\end{tabularx}
\end{small}
\end{table}

\begin{proposition}\label{prop:cq}
The problem of finding a universal solution is PTime for CQs with negation. 
\end{proposition}

\begin{proof}
Given a CQ $Q$, its universal solution is composed of a single c-instance that contains all tables that appear in $Q$. For each positive atom of $Q$, we add a tuple in the appropriate table and for each negated atom or selection condition, we add it to the global condition. 
This c-instance satisfies $Q$ and covers all atoms of $Q$. Therefore, it is a universal solution.
\end{proof}


\begin{proposition}
The problem of finding a universal solution is \#P-complete for UCQs with negation. 
\end{proposition}

\begin{proof}
\amir{Verify:}
We first show that the problem belongs in \#P by showing that the problem of finding the c-instances in the universal solution is equivalent to counting the number of satisfying assignment to the UCQ. 
Let $Q = q_1 \lor \ldots \lor q_r$ be a UCQ. 
Note that each satisfying c-instance of $Q$ must cover a subset of $\{q_1, \ldots, q_r\}$, where for each $q_i$ it must cover all atoms of $q_i$ (recall the proof of Proposition \ref{prop:cq}). 
A universal solution can be found if we can count the number of minimal satisfying c-instances 
% with covers that are not contained in each other 
(these are exactly the c-instances in the universal solution). 
Each subset of satisfied CQs $S \subseteq \{q_1, \ldots, q_r\}$ can only have a single assignment satisfying it (as all CQs in $S$ have to be satisfied at once so this is essentially a conjunction of CQs).
Thus, $S$ defines exactly one c-instance in the universal solution, since this is equivalent to the universal solution of a CQ (again, recall the proof of Proposition \ref{prop:cq}). 
Therefore, the number of c-instances in the universal solution is equivalent to the number satisfying assignments to $Q$ and generating a c-instance for each one in PTime as shown in Proposition \ref{prop:cq}. 
% and then comparing each pair of c-instances $\cinstance_1,\cinstance_2$ and removing $\cinstance_1$ from the set if all of the CQs satisfied by $\cinstance_1$ are also satisfied by $\cinstance_2$. 

We prove hardness by reduction from counting the satisfying assignments to a DNF formula, known to be \#P-complete. 
Given a DNF formula $\phi = \varphi_1 \lor \ldots \lor \varphi_k$, we generate the Boolean query $Q$ whose formula is 
% $\phi = \varphi_1 \lor \ldots \lor \varphi_k$. 
$R(x_1) \land \neg R(x_2) \land R(x_3)$ for every clause $\varphi = (x_1 \land \neg x_2 \land x_3)$ and a $\lor$ connecting the clauses of $Q$. 
We claim that each satisfying assignment to $Q$, $\alpha$, can be mapped to a c-instance in the universal solution $\{\cinstance_1, \ldots, \cinstance_l\}$. 
Given a satisfying assignment $\alpha$, its coverage is exactly the number of literals whose value is mapped to True. Assume $\alpha$ satisfies the clauses $\varphi_i \ldots \varphi_j$, and in particular, {\em all literals in these clauses are evaluated to True}. 
In the universal solution, there is a c-instance $\cinstance$ that satisfies $\varphi_i \ldots \varphi_j$ and possibly more clauses. So, in $\cinstance$, the literals in $\varphi_i \ldots \varphi_j$ are all evaluated to True. Since $\phi$ is a DNF, every assignment that satisfies a subset of the clauses satisfies $\phi$.  
Thus, $\cinstance$ encodes every assignment that satisfies a subset of the clauses that it satisfies. 
% To check the assignments encoded in $\cinstance$, we can go over each of the clauses, satisfy all of the literals in it and check which other clauses have also been satisfied in the process 
% (since $\phi$ is a DNF, every clause can be satisfied in exactly one manner - satisfying all literals in it). 
Therefore, we can count the number of satisfying assignments by counting the number of subsets of clauses satisfied by each c-instance in the universal solution. 
% For the other direction, given all satisfying assignments,
\end{proof}


\subsection{Pseudo Code for Algorithms in Section \ref{sec:disjunct}}

\begin{algorithm}[h]\caption{Handle-Or-Operator}\label{alg:or-op}
  \centering
{\small
\begin{codebox}
  \Procname{$\proc{Handle-Or}(\schemaOf{\rel}, Q, I, f)$}
    \li ConjTrees $\gets \proc{Expand-DisjTree}(Q.root)$
    \li \For $T \in ConjTrees$
    \Do
        \li res.extend($\proc{Tree-Chase-BFS}($\schemaOf{\rel}$, T, I, f)$)
    \End
\li \Return $res$
\end{codebox}
}
\end{algorithm}


\begin{algorithm}[h]\caption{Handle-Existential-Operator}\label{alg:exists-op}
  \centering
{\small
\begin{codebox}
    \li \For $x \in I.domain(Q.root.variable)$
    \Do
        \li $g \gets f \cup \{Q.root.variable \to x\}$
        \li res.extend($\proc{Tree-Chase-BFS}(\schemaOf{\rel}, Q.root.child, I, g, limit)$)
    \End
    \li Create a fresh labeled null $y$ in the domain of $Q.root.variable$\label{alg:rd-tree-chase:line:exists-add-fresh-start}
    \li $g \gets f \cup \{Q.root.variable \to y\}$
    \li $I.domain(Q.root.variable) \gets I.domain(Q.root.variable) \cup \{y\}$
    \li res.extend($\proc{Tree-Chase-BFS}(\schemaOf{\rel}, Q.root.child, I, g, limit)$)\label{alg:rd-tree-chase:line:exists-add-fresh-end}
\li \Return $res$
\end{codebox}
}
\end{algorithm}


\input{sections/completeness_proof}
\input{sections/all_queries}
